# Supplementary material for: Electronic Physics and Possible Superconductivity in Layered Orthorhombic Cobalt Oxychalcogenides
Source: arXiv:1612.03470 source file (2016-12-11)
Supplement: Supplementary file 1 [file BaCoSO_supplementary.pdf]

# Supplementary

(Dated: December 10, 2016)

PACS numbers: 75.85.+t, 75.10.Hk, 71.70.Ej, 71.15.Mb

In this supplementary, we provide the details about the calculations and methods of the paper. In the first section, the detailed crystal structures of BaCoAO(A=S,Se) are given. In the second section, we discuss the effective tight binding models. Finally, we discuss the mean-field calculations for the superconducting state.

## I. METHODS AND CRYSTAL STRUCTURE

Our density functional theory calculations employ the projector augmented wave (PAW) method encoded in Vienna ab initio simulation package(VASP)[1–3], and the generalized-gradient approximation (GGA) for the exchange correlation functional is used[4]. The cutoff energy of 550 eV is taken for expanding the wave functions into the plane-wave basis. In the calculation for monolayer BaCoAO(A=S,Se), the number of these k points is $(7 \times 11 \times 3)$ for the nonmagnetic calculations and $(7 \times 6 \times 3)$ for the magnetic calculations. The GGA plus on-site repulsion U method (GGA+U) in the formulation of Dudarev *et al.*[5] is employed to describe the electron correlation effect associated with the Co $3d$ states by an effective parameter $U_{eff}$. The value of $U_{eff} = 3eV$ on Co is adopted in the calculations. We relax the lattice constants and internal atomic positions with GGA, where the plane wave cutoff energy is 600eV. Forces are minimized to less than 0.01 eV/Å in the relaxation.

The crystal structure of bulk BaCoSO with the space group Cmcm is isostructural to BaZnSO, shown in the main text. The local environment of Co is a tetrahedra being formed by two sulfur and two oxygen ions, similar to the environment of Fe in iron-based superconductors. The puckered layers are constructed by vertex-shared tetrahedra cation-anion complexes. In order to simplify calculations, we focus on the monolayer BaCoAO(A=S,Se). Table.S1 lists the optimized structural parameters of the monolayer BaCoAO(A=S,Se). The optimized structural parameters of the monolayer BaCoSO are close to these of the bulk BaCoSO.

TABLE S1: Experimental and Optimized structural parameters of the monolayer BaCoAO(A=S,Se) by the GGA in the paramagnetic phase.

| | BaCoSO | BaCoSeO | bulk BaCoSO[6] |
|---|---|---|---|
| a(Å) | 5.940 | 5.972 | 6.107 |
| b(Å) | 3.850 | 3.895 | 3.988 |
| c(Å) | 15.000 | 15.000 | 12.755 |
| Co-S/Se(Å) | 2.181 | 2.340 | 2.336 |
| Co-O(Å) | 1.963 | 1.939 | 1.941 |
| $\alpha$(S/Se-Co-S/Se) | 123.879° | 112.667° | 116.994° |
| $\beta$(O-Co-O) | 98.274° | 100.716° | 103.434° |

## II. TIGHT BINDING MODELS

The d orbitals of Co atoms are responsible for electronic physics in these systems. The effective tight binding model Hamiltonian $H_0$ to describe the band structure of monolayer BaCoAO(A=S,Se) can be written as a 5×5 Hermitian matrix by choosing one Co unit cell as discussed in the main text. The noninteracting Hamiltonian is $H = \sum_{\mathbf{k}\sigma} \phi^\dagger_{\mathbf{k}\alpha\sigma} h(\mathbf{k}) \phi_{\mathbf{k}\alpha\sigma}$, where $\phi^\dagger_{\mathbf{k}\alpha\sigma} = [c^\dagger_{d_{z^2}\sigma}(\mathbf{k}), c^\dagger_{d_{xz}\sigma}(\mathbf{k}), c^\dagger_{d_{yz}\sigma}(\mathbf{k}), c^\dagger_{d_{x^2-y^2}\sigma}(\mathbf{k}), c^\dagger_{d_{xy}\sigma}(\mathbf{k})]$ are creation operators for electrons in $d$ orbitals with spin $\sigma$. The elements of $H_0$ matrix are given by

$$\begin{aligned}
H_{11} &= \epsilon_1 + 2t_x^{11}cos(2k_x) + 2t_y^{11}cos(k_y) + 2t_{yy}^{11}cos(2k_y) \\
&\quad + 2t^{16}cos(k_x) + 4t_y^{16}cos(k_x)cos(k_y), \\
H_{12} &= 2it_x^{12}sin(2k_x) - 2it^{17}sin(k_x) - 4it_y^{17}sin(k_x)cos(k_y) \\
H_{13} &= 2it_y^{13}sin(k_y) + 2it_{yy}^{13}sin(2k_y) - 4it_y^{18}cos(k_x)sin(k_y) \\
H_{14} &= 2t_x^{14}cos(2k_x) + 2t_y^{14}cos(k_y) + 2t_{yy}^{14}cos(2k_y) \\
&\quad + 2t^{19}cos(k_x) + 4t_y^{19}cos(k_x)cos(k_y) \\
H_{15} &= -4t_y^{110}sin(k_x)sin(k_y) \\
H_{22} &= \epsilon_2 + 2t_x^{22}cos(2k_x) + 2t_y^{22}cos(k_y) + 4t_{yy}^{22}cos(2k_y) \\
&\quad - 2t^{27}cos(k_x) - 4t_y^{27}cos(k_x)cos(k_y), \\
H_{23} &= 4t_y^{28}sin(k_x)sin(k_y) \\
H_{24} &= 2it_x^{24}sin(2k_x) + 2it^{29}sin(k_x) + 4it_y^{29}sin(k_x)cos(k_y) \\
H_{25} &= 2it_y^{25}sin(k_y) + 2it_{yy}^{25}sin(2k_y) + 4it_y^{210}cos(k_x)sin(k_y) \\
H_{33} &= \epsilon_3 + 2t_x^{33}cos(2k_x) + 2t_y^{33}cos(k_y) + 2t_{yy}^{33}cos(2k_y) \\
&\quad - 2t^{38}cos(k_x) - 4t_y^{38}cos(k_x)cos(k_y), \\
H_{34} &= 2it_y^{34}sin(k_y) + 2it_{yy}^{34}sin(2k_y) + 4it_y^{39}cos(k_x)sin(k_y) \\
H_{35} &= 2it_x^{35}sin(2k_x) + 2it^{310}sin(k_x) + 4it_y^{310}sin(k_x)cos(k_y) \\
H_{44} &= \epsilon_4 + 2t_x^{44}cos(2k_x) + 2t_y^{44}cos(k_y) + 2t_{yy}^{44}cos(2k_y) \\
&\quad + 2t^{49}cos(k_x) + 4t_y^{49}cos(k_x)cos(k_y), \\
H_{45} &= -4t_y^{410}sin(k_x)sin(k_y) \\
H_{55} &= \epsilon_5 + 2t_x^{55}cos(2k_x) + 2t_y^{55}cos(k_y) + 2t_{yy}^{55}cos(2k_y) \\
&\quad + 2t^{510}cos(k_x) + 4t_y^{510}cos(k_x)cos(k_y),
\end{aligned} \tag{1}$$

where $\epsilon$ are the onset energy of the $d$ orbitals. Table.S2 shows the corresponding hopping parameters in the above questions for the monolayer BaCoAO(A=S,Se) above equation. Fig.S1(a) and (b) display the band structure from the DFT calculations and tight binding bands. They match well with each other near the Fermi level.

As the $t_{2g}$ orbitals dominates near Fermi energy, we can further simplify the above effective Hamiltonian by only using of

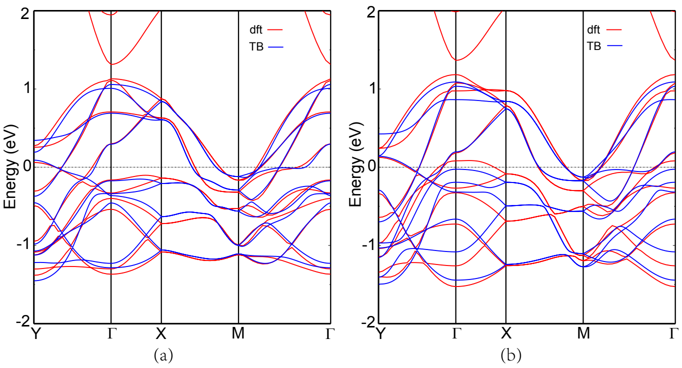


FIG. S1: (color online) The band structures from the DFT and the five-orbital tight binding models for (a) BaCoSeO and (b) BaCoSO.

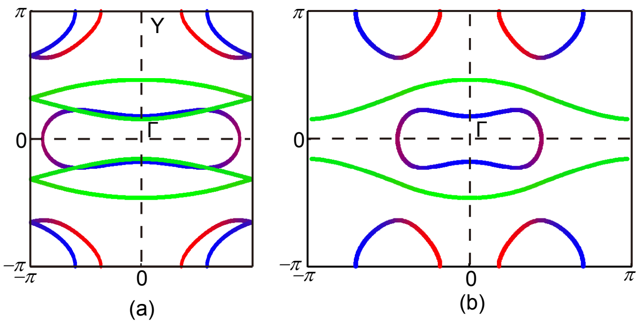


FIG. S2: (color online) (a) Fermi surface and (b) the unfold Fermi surface of the three-orbital model. The orbital contributions of the different FS sheets are shown with coded colors: $d_{xz}$(red), $d_{yz}$ (green) and $d_{x^2-y^2}$ (bule).

TABLE S2: The hopping parameters to fit the DFT bands in the tight binding model for the monolayer BaCoSO(BaCoSeO). The on-site energies of the five d orbitals are (all in eV): $\epsilon_1$ = -0.722(-0.89), $\epsilon_2$ = -0.297(-0.405), $\epsilon_3$ = -0.557(-0.521), $\epsilon_4$ = -0.328(-0.463), and $\epsilon_5$ = -0.832( -0.886).

| $t_i^{mn}$ | i=0 | i=x | i=y | i=yy |
|---|---|---|---|---|
| mn=11 | | -0.03(-0.032) | 0.133(0.04) | -0.023(-0.018) |
| mn=12 | | -0.036(-0.033) | | |
| mn=13 | | | 0.072(0.159) | 0.018(-0.019) |
| mn=14 | | 0.002(0.003) | 0.226(0.162) | -0.02(-0.014) |
| mn=16 | -0.154(-0.182) | | 0.006(0.012) | |
| mn=17 | 0.121(0.104) | | 0.0148(0.008) | |
| mn=18 | | | -0.02(-0.009) | |
| mn=19 | 0.094(0.12) | | -0.022(-0.019) | |
| mn=110 | | | 0.007(-0.001) | |
| mn=22 | | 0.051(0.053) | 0.207(0.191) | -0.012(-0.018) |
| mn=24 | | -0.002(-0.006) | | |
| mn=25 | | | -0.221(-0.179) | 0.01(-0.015) |
| mn=27 | -0.323(-0.329) | | -0.014(-0.007) | |
| mn=28 | | | 0.025(0.016) | |
| mn=29 | 0.137(0.115) | | 0.033(0.028) | |
| mn=210 | | | -0.02(-0.016) | |
| mn=33 | | -0.014(-0.022) | 0.412(0.378) | 0.077(0.086) |
| mn=34 | | | 0.093(-0.035) | 0.012(-0.02) |
| mn=35 | | -0.016(-0.02) | | |
| mn=38 | -0.204(-0.23) | | -0.003(0.02) | |
| mn=39 | | | -0.051(-0.04) | |
| mn=310 | 0.155(0.18) | | 0.017(0.002) | |
| mn=44 | | -0.018(-0.013) | 0.2(0.202) | -0.037(-0.041) |
| mn=49 | -0.275(-0.25) | -0.014(-0.016) | | |
| mn=410 | | | 0.035(0.025) | |
| mn=55 | 0.029(0.028) | -0.244(-0.172) | | 0.01(0.013) |
| mn=510 | -0.152(-0.172) | | -0.022(-0.018) | |

TABLE S3: The hopping parameters to fit the DFT bands in the three orbital tight binding model for monolayer BaCoSO. The on-site energies of the d oribtals are (all in eV): $\epsilon_2$ = -0.405, $\epsilon_3$ = -0.507, $\epsilon_4$ =-0.178.

| $t_i^{mn}$ | i=0 | i=x | i=y | i=yy |
|---|---|---|---|---|
| mn=22 | | 0.051 | 0.207 | -0.012 |
| mn=24 | | -0.002 | | |
| mn=27 | -0.323 | | -0.014 | |
| mn=28 | | | 0.025 | |
| mn=29 | 0.137 | | 0.033 | |
| mn=33 | | -0.014 | 0.412 | 0.077 |
| mn=34 | | | 0.093 | 0.012 |
| mn=38 | -0.204 | | -0.003 | |
| mn=39 | | | -0.051 | |
| mn=44 | | -0.028 | 0.22 | 0.033 |
| mn=49 | -0.225 | 0.026 | | |

the three $t_{2g}$ orbitals. Thus, the minimum effective model is a 3×3 Hermitian matrix constructed by the three $t_{2g}$ orbitals. We take ($d_{xz}$, $d_{yz}$,$d_{x^2-y^2}$) as the basis in the minimum effective model, and the elements of $H_0$ matrix are given by

$$
\begin{aligned}
H_{11} &= \epsilon_2 + 2t_x^{22}cos(2k_x) + 2t_y^{22}cos(k_y) + 4t_{yy}^{22}cos(2k_y) \\
&\quad -2t^{27}cos(k_x) - 4t_y^{27}cos(k_x)cos(k_y), \\
H_{12} &= 4t_y^{28}sin(k_x)sin(k_y) \\
H_{13} &= 2it_x^{24}sin(2k_x) + 2it^{29}sin(k_x) + 4it_y^{29}sin(k_x)cos(k_y) \\
H_{22} &= \epsilon_3 + 2t_x^{33}cos(2k_x) + 2t_y^{33}cos(k_y) + 2t_{yy}^{33}cos(2k_y) \\
&\quad -2t^{38}cos(k_x) - 4t_y^{38}cos(k_x)cos(k_y), \\
H_{23} &= 2it_y^{34}sin(k_y) + 2it_{yy}^{34}sin(2k_y) + 4it_y^{39}cos(k_x)sin(k_y) \\
H_{33} &= \epsilon_4 + 2t_x^{44}cos(2k_x) + 2t_y^{44}cos(k_y) + 2t_{yy}^{44}cos(2k_y) \\
&\quad +2t^{49}cos(k_x) + 4t_y^{49}cos(k_x)cos(k_y),
\end{aligned}
$$

where $\epsilon$ are the onset energy of the $d$ orbitals. Table.S3 shows the corresponding hopping parameters of the model for the monolayer BaCoSO. Fit.**??** plots the folded and unfolded band structures from the three orbital models. **Plot the band structure of the three orbital models.** Fig.S2(a) and (b) display the Fermi surface of the three orbital model at three different doping regions **Plot similar three Fermi surfaces as those from the 5 orbital model in main text** in folded and unfolded BZ. The three orbitals well capture the Fermi surfaces attributed to the $t_{2g}$ orbitals.

## III. THE MEAN FIELD RESULTS FOR THE SC STATE

We carry out the mean field calculation for the superconducting states of BaCoSO based on the t-J model and analyze qualitative results on superconducting order parameters. The t-J Hamiltonian after the mean-field treatment can be written as

$$H_{eff} = H_0' + \sum_{\langle i,j\rangle,\alpha} J^{\alpha}_{ab}(\mathbf{S}_{i,a} \cdot \mathbf{S}_{j,b} - \frac{1}{4} n_{i,a} n_{j,b}), \quad (2)$$

where $H_0'$ is taken to be the renormalized band structure. In the mean-field treatment, $H_0'$ can be approximated to be proportional to the bare band structure $H_0$. Therefore, for qualitative results on superconducting order parameters, we can simply use $H_0$ in our calculations for $H_0'$ in Eq.2. As the Fermi surfaces are mainly contributed from the three $t_{2g}$ orbitals and the intra-orbital AFM couplings are expected to be dominant, we simplify the AFM interaction terms in Eq.3 as

$$\sum_{\langle i,j\rangle,\alpha,a\in t_{2g}} J^{\alpha}_{a}(\mathbf{S}_{i,a} \cdot \mathbf{S}_{j,a} - \frac{1}{4} n_{i,a} n_{j,a}). \quad (3)$$

For simplicity, we ignore the difference among three $t_{2g}$ orbitals. We choose the AFM coupling terms as $J^x_a = 0.8 * J^y_a = J$ and $J^{\alpha}_a = J^{\alpha}_b$ for all of the three $t_{2g}$ orbitals. By decoupling the AFM interactions in the pairing channels, we define the superconducting order parameters as

$$\Delta^{\alpha}_a = J^{\alpha} < c^{+}_{i,a,\uparrow} c^{+}_{i+\delta_\alpha,a,\downarrow} >, \quad (4)$$

where $\delta_\alpha$ are unit lattice vectors along two directions. For a uniform superconducting state, $\Delta^{\alpha}_a$ does not depend on site. The results are reported in Fig.S3.

In all the parameter regions, we find that in the mean-field calculations, the SC order parameters for $xz$ orbital and $yz$ orbital are both d-wave like, while it is s-wave like for $x^2 - y^2$ orbital. Namely, $sign(\Delta^x_{xz}) = -sign(\Delta^y_{xz})$, $sign(\Delta^x_{yz}) = -sign(\Delta^y_{yz})$ and $sign(\Delta^x_{x^2-y^2}) = sign(\Delta^y_{x^2-y^2})$. Furthermore, if we check the pairing order parameter carefully for each $t_{2g}$ orbital, it can be found that, in a physical parameter region that $J_x$ is smaller than $0.7eV$, $sign(\Delta^x_{xz}) = -sign(\Delta^y_{yz}) = sign(\Delta^x_{x^2-y^2})$. This result suggests that the superconducting state is a d-wave like state.

The SC gap reported in the main text is under the parameter $J_x = 0.8J_y = 0.4eV$. The corresponding SC order parameters are $\Delta^x_{xz} = -0.0446eV$, $\Delta^x_{yz} = -0.0303eV$, $\Delta^x_{x^2-y^2} = 0.0346eV$ in the x-direction, and $\Delta^y_{xz} = 0.0920eV$, $\Delta^y_{yz} = 0.0762eV$, $\Delta^y_{x^2-y^2} = 0.0825eV$ in the y-direction.


[1] G. Kresse and J. Hafner, Phys. Rev. B **47**, 558 (1993).

[2] G. Kresse and J. Furthmuller, Comput. Mater. Sci. **6**, 15 (1996).

[3] G. Kresse and J. Furthmuller, Phys. Rev. B **54**, 11169 (1996).

[4] J. P. Perdew, K. Burke, and M. Ernzerhof, Phys. Rev. Lett. **77**, 3865 (1996).

[5] S. L. Dudarev, G. A. Botton, S. Y. Savrasov, C. J. Humphreys, and A. P. Sutton, Phys. Rev. B **57**, 1505 (1998).

[6] Martin Valldor, Ulrich K. Robler, Yurii Prots, Chang-Yang Kuo, Jen-Che Chiang, Zhiwei Hu, Tun-Wen Pi, Rdiger Kniep, and Liu Hao Tjeng, Chemistry-A European Journal, 2015, 21(30): 10821-10828.

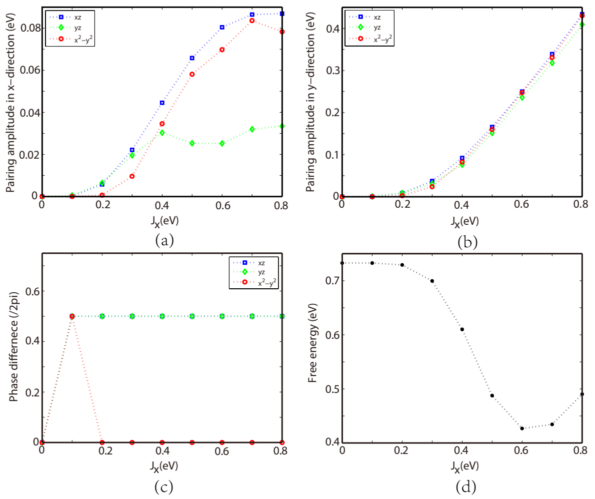


FIG. S3: (color online) The mean field results for BaCoSO. In the mean field calculations, the AFM coupling has been set to be $J_x = 0.8J_y$. (a) and (b) show the pairing amplitude in x-direction and y-direction, respectively. The phase difference between $\Delta^x$ and $\Delta_y$ for each $t_{2g}$ orbital is shown in (c), and the free energy is presented in (d).
